# Supplementary material for: Derivation of the Biot-Savart equation from the Nonlinear Schr\"odinger equation
Source: arXiv:1507.07806 source file (2016-04-21)
Supplement: Supplementary file 1 [file Supplemental_Material_NLS.pdf]

# Equations and integrals for NLS Biot-Savart paper. Miguel Bustamante, UCD, 2015

## Contents:
(1) Numerical Solution for Pitaevskii vortex profile R(r).
(2) Application of this solution to compute cut-off length $\xi_*$ and other integrals.

### Equation of motion for profile R[r]:

```
eqψ = FullSimplify[(R[r] Exp[I θ] + Exp[I θ] * 1 / r D[r R'[r], r] +
    R[r] * 1 / r^2 D[Exp[I θ], θ, θ] - Exp[I θ] R[r]^3) ⅇ^(-ⅈ θ)]
```

$$R[r] - \frac{R[r]}{r^2} - R[r]^3 + \frac{R'[r]}{r} + R''[r]$$

```
ρPade[r_] := r^2 (0.3437 + 0.0286 r^2) / (1 + 0.3333 r^2
+ 0.0286 r^4)
```

### Asymptotic expansion, large r: $R[r] = \mathrm{Exp}\left[Z\left[\frac{1}{r^2}\right]\right]$. Function RAsymNew[11][r] will be used for the construction of the full numerical function.

$$\text{eqInf[u\_]} := -1 + \frac{1 - e^{2 Z[u]}}{u} + 4\, u\, Z'[u] + 4\, u^2\, Z'[u]^2 + 4\, u^2\, Z''[u]$$

```
Ztemp[u_] := -Sum[coef[j] u^j, {j, 1, 15}]

polyUtemp = Normal[Series[eqInf[u] /. Z → Ztemp, {u, 0, 15}]];

solCoef = {}; Do[solCoef = Join[solCoef,
   Solve[(CoefficientList[polyUtemp, u][[j]] /. solCoef) == 0][[1]]], {j, 1, 15}]

solCoef
```

$$\Big\{\text{coef}[1] \to \frac{1}{2},\ \text{coef}[2] \to \frac{5}{4},\ \text{coef}[3] \to \frac{32}{3},\ \text{coef}[4] \to \frac{1589}{8},\ \text{coef}[5] \to \frac{64\,981}{10},$$
$$\text{coef}[6] \to \frac{989\,939}{3},\ \text{coef}[7] \to \frac{168\,211\,250}{7},\ \text{coef}[8] \to \frac{38\,006\,710\,085}{16},$$
$$\text{coef}[9] \to \frac{5\,510\,235\,057\,787}{18},\ \text{coef}[10] \to \frac{199\,454\,257\,136\,329}{4},$$
$$\text{coef}[11] \to \frac{110\,192\,683\,498\,843\,556}{11},\ \text{coef}[12] \to \frac{14\,600\,012\,068\,277\,445\,755}{6},$$
$$\text{coef}[13] \to \frac{9\,139\,380\,150\,115\,822\,460\,510}{13},\ \text{coef}[14] \to \frac{1\,667\,906\,914\,654\,942\,805\,513\,414}{7},$$
$$\text{coef}[15] \to \frac{1\,404\,358\,943\,944\,993\,346\,402\,456\,342}{15}\Big\}$$

```
Clear[RAsym]
```

```
RAsym[r_] := Exp[Ztemp[1 / r^2] /. solCoef]
```

```
Clear[RAsymNew]
```

```
RAsymNew[k_][r_] := Exp[-Sum[coef[j] r^(-2 j), {j, 1, k}] /. solCoef]
```

```
RAsym[r]
```

$$e^{-\frac{1404358943944993346402456342}{15 r^{30}}-\frac{1667906914654942805513414}{7 r^{28}}-\frac{9139380150115822460510}{13 r^{26}}-\frac{14600012068277445755}{6 r^{24}}-\frac{110192683498843556}{11 r^{22}}-\frac{199454257136329}{4 r^{20}}-\frac{5\text{[illegible]}}{}}$$

```
Plot[Evaluate[RAsymNew[8][r]], {r, 5, 100}, PlotRange → {0, 1}]
```

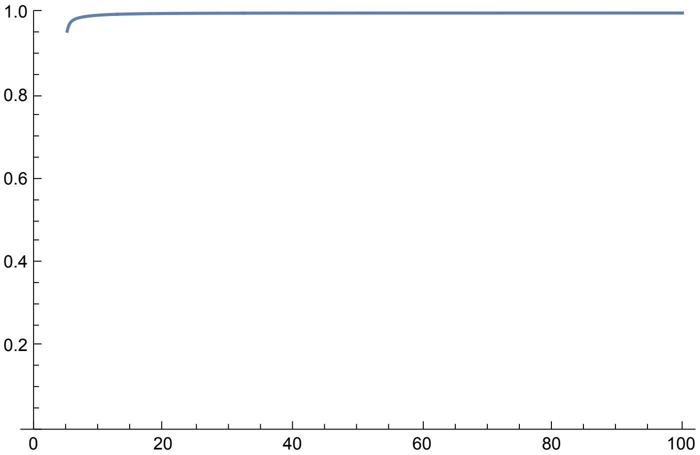


```
Plot[Evaluate[RAsym[r]], {r, 5, 100}, PlotRange → {0, 1}]
```

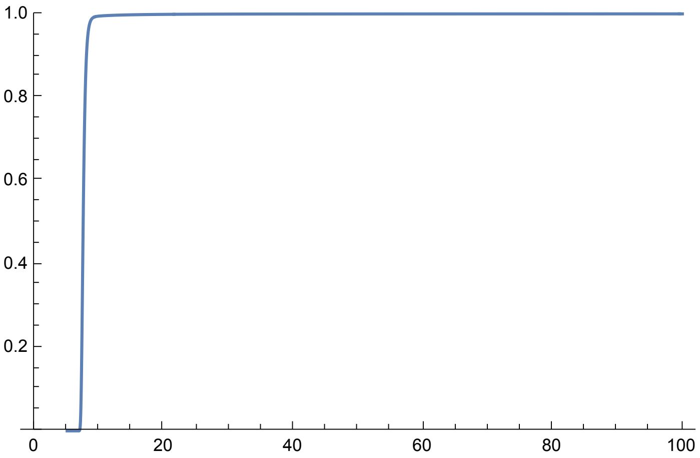


## Numerical simulation “shooting” method to find R[r].

Explanation of input:
**orderAsym** denotes the number of terms in the asympototic expansion.
**prec** denotes the required precision and accuracy goals, as well as the working precision for the numerical solution method for the ODE for R[r].
**L0** denotes minus the logarithm of the initial position $r_0$ ($\ll 1$) for the solution of the ODE for R[r].
**fTempRNew[a]** is a function that takes the value **a** of tentative initial slope of function R[r] at r = $r_0$. It produces the three functions R[r], R’[r] and R’’[r] over a certain range, as interpolating functions.

Explanation of output:
**solAllRTemp** is the output of fTempRNew[a].
**Plot** of the three functions R[r], R’[r], R’’[r] as function of r. Blue: R[r].
**rTrans** is the position r at which the numerical solution for R[r], denoted solAllRTemp[[1]], coincides

with the asymptotic solution RAsymNew[orderAsym][r].
**“difference”** denotes the jump in the function R[r] at r = rTrans between RAsymNew[orderAsym][r] and solAllRTemp[[1]].
**“absolute error”** denotes the jump in the derivative function R’[r] at r = rTrans between RAsymNew[orderAsym][r] and solAllRTemp[[1]].
**“relative error”** denotes the relative jump in the derivative function R’[r] at r = rTrans between RAsymNew[orderAsym][r] and solAllRTemp[[1]].

```
orderAsym = 13;
prec = 22;
L0 = 50`24;
fTempRNew[a_] := NDSolveValue[{-R[r] + r^2 R[r] - r^2 R[r]^3 + r R′[r] + r^2 R′′[r] == 0,
    R[Exp[-L0]] == Exp[-L0] * a, R'[Exp[-L0]] == a}, {R[r], R'[r], R''[r]},
   {r, Exp[-L0], 30}, Method → "StiffnessSwitching", WorkingPrecision → prec,
   MaxSteps → 600, AccuracyGoal → 22, PrecisionGoal → 22,
   StartingStepSize → 10^-21, InterpolationOrder → 22];
solAllRTemp = fTempRNew[0.5831894958603292791791737551`24];
{Plot[solAllRTemp, {r, 0., 30.}, PlotRange → {0, 1}, ImageSize → Medium],
 rTrans = r /. FindRoot[(solAllRTemp[[1]]) - RAsymNew[orderAsym][r] == 0,
    {r, 18.5}, WorkingPrecision → prec];
 MatrixForm[{"rTrans=", rTrans, "difference=",
   ((solAllRTemp[[1]]) - RAsymNew[orderAsym][r]) /. r → rTrans}], MatrixForm[
  {"absolute error=", ((solAllRTemp[[2]]) - RAsymNew[orderAsym]'[r]) /.
    r → rTrans, "relative error=",
   ((solAllRTemp[[2]]) / RAsymNew[orderAsym]'[r] - 1) /. r → rTrans}]}
```

{ 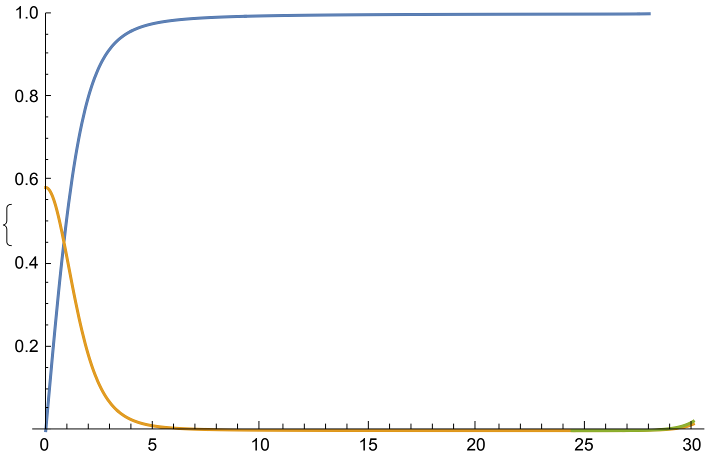 ,

$\begin{pmatrix} \text{rTrans=} \\ 15.57522386121755965633 \\ \text{difference=} \\ 0. \times 10^{-22} \end{pmatrix}$ , $\begin{pmatrix} \text{absolute error=} \\ -1.207079951 \times 10^{-15} \\ \text{relative error=} \\ -4.47261686 \times 10^{-12} \end{pmatrix}$ }

## Plots for further analysis:

```
Plot[Evaluate[{(solAllRTemp[[1]]) - RAsymNew[orderAsym][r]}],
 {r, 12, 17}, PlotRange → All, WorkingPrecision → prec]
```

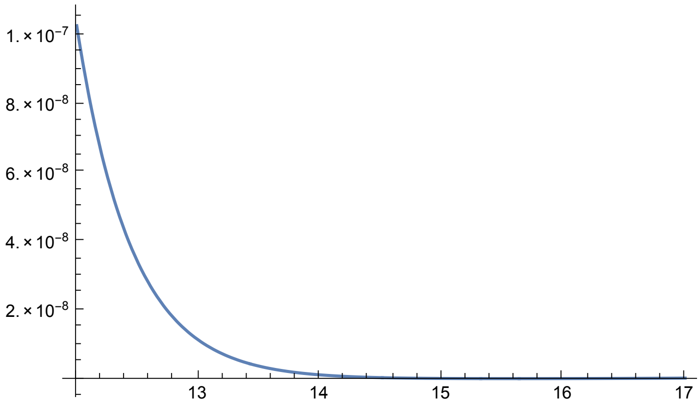


```
rTrans = r /. FindRoot[(solAllRTemp[[1]]) - RAsymNew[orderAsym][r] == 0,
   {r, 18.5}, WorkingPrecision → prec]
```

15.575223861217559656 33

```
((solAllRTemp[[1]]) - RAsymNew[orderAsym][r]) /. r → rTrans
```

$0. \times 10^{-22}$

## Jump in the derivative of vortex profile R(r):
## Absolute:

```
((solAllRTemp[[2]]) - RAsymNew[orderAsym]'[r]) /. r → rTrans
```

$-1.207079951 \times 10^{-15}$

## Relative:

```
((solAllRTemp[[2]]) / RAsymNew[orderAsym]'[r] - 1) /. r → rTrans
```

$-4.47261686 \times 10^{-12}$

## Pade approximation:

```
RPade[r_] := Sqrt[ρPade[r]]
```

# Errors: plotting the LHS of the ODE for R[r], using the different approximate functions.

## Error in Pade:

```
LogLogPlot[Abs[((R[r] - R[r]/r^2 - R[r]^3 + R′[r]/r + R″[r]) // Expand) /. R → RPade],
 {r, 10^-17, 10^-8}, PlotRange → All]
```

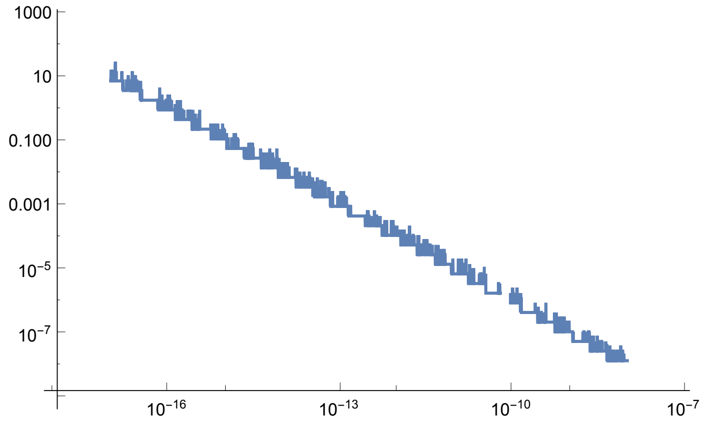


```
LogLogPlot[Abs[((R[r] - R[r]/r^2 - R[r]^3 + R′[r]/r + R″[r]) // Expand) /. R → RPade],
 {r, 10^-8, 10^1}, PlotRange → All]
```

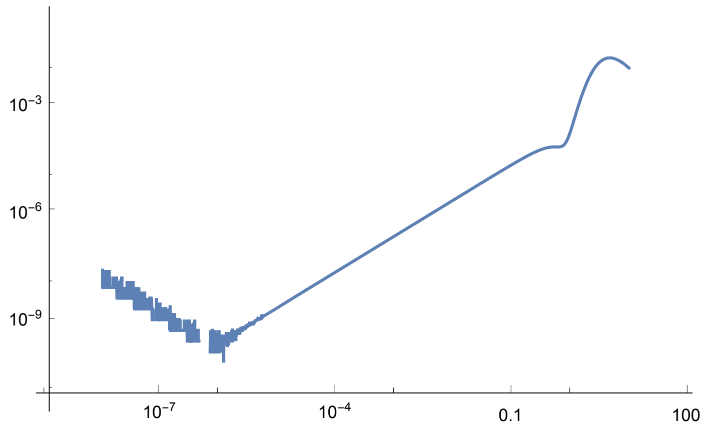

```
LogLogPlot[Abs[((R[r] - R[r]/r^2 - R[r]^3 + R'[r]/r + R''[r]) // Expand) /. R → RPade],
 {r, 10^1, 10^3}, PlotRange → All]
```

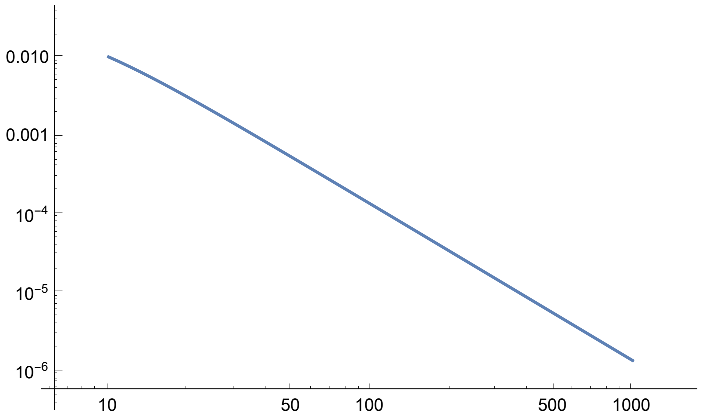


## Error in large-r asymptotic solution **RAsymNew[orderAsym][r]**:

```
Plot[Evaluate[(R[r] - R[r]/r^2 - R[r]^3 + R'[r]/r + R''[r]) /. R :> RAsymNew[orderAsym]],
 {r, 14.5, 100}, PlotRange → All, WorkingPrecision → 30]
```

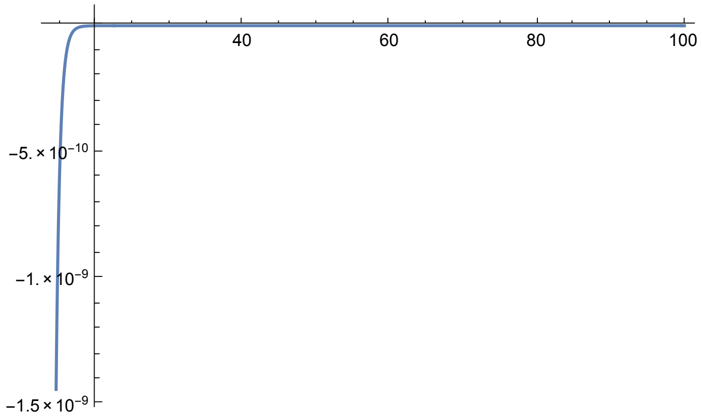

## Error in numerical solution **solAllRTemp:**

```
LogLinearPlot[Evaluate[(R - R/r^2 - R^3 + Rp/r + Rpp) /.
    {R → solAllRTemp[[1]], Rp → solAllRTemp[[2]], Rpp → solAllRTemp[[3]]}],
  {r, 10^-17, 10^-6}, WorkingPrecision → 45, PlotRange → {-10^-13, 10^-13},
  MaxRecursion → 10, PlotPoints → 1000]
```

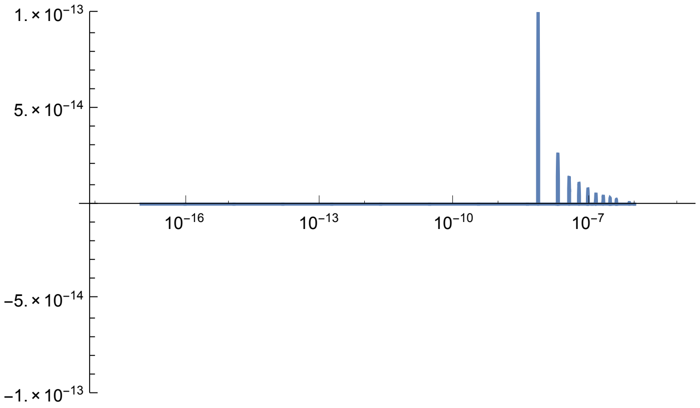


```
LogLinearPlot[Evaluate[(R - R/r^2 - R^3 + Rp/r + Rpp) /.
    {R → solAllRTemp[[1]], Rp → solAllRTemp[[2]], Rpp → solAllRTemp[[3]]}],
  {r, 10^-6, 10^-4}, WorkingPrecision → 38, PlotRange → {-10^-15, 10^-15},
  MaxRecursion → 15, PlotPoints → 1000]
```

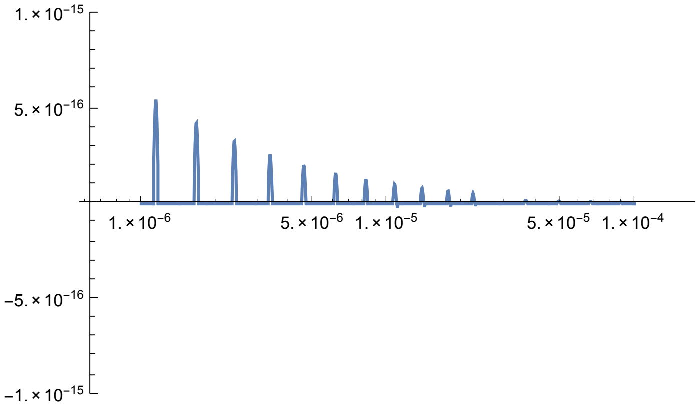

```
LogLinearPlot[Evaluate[(R - R/r^2 - R^3 + Rp/r + Rpp) /.
    {R → solAllRTemp[[1]], Rp → solAllRTemp[[2]], Rpp → solAllRTemp[[3]]}],
  {r, 10^-4, 10^-2}, WorkingPrecision → 30, PlotRange → {-10^-17, 10^-17},
  MaxRecursion → 15, PlotPoints → 1000]
```

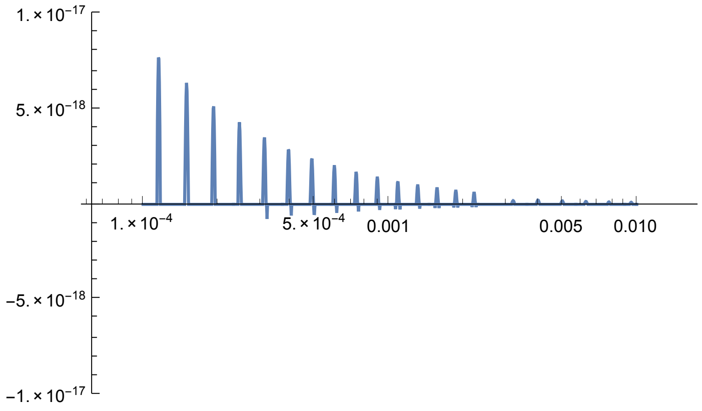


```
LogLinearPlot[Evaluate[(R - R/r^2 - R^3 + Rp/r + Rpp) /.
    {R → solAllRTemp[[1]], Rp → solAllRTemp[[2]], Rpp → solAllRTemp[[3]]}],
  {r, 10^-2, 1}, WorkingPrecision → 30, PlotRange → {-10^-19, 10^-19},
  MaxRecursion → 15, PlotPoints → 1000]
```

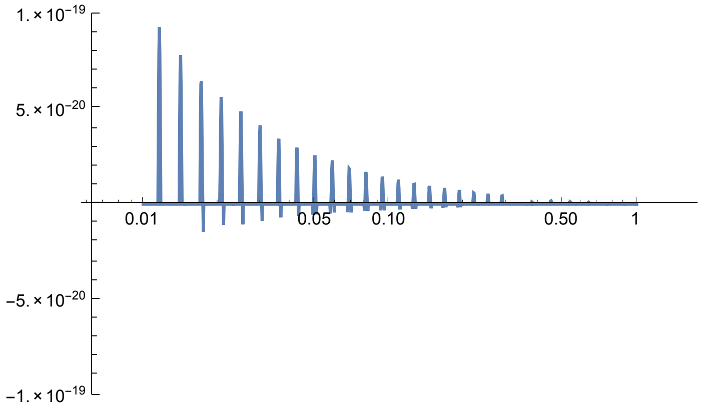

```
LogLinearPlot[Evaluate[(R - R/r^2 - R^3 + Rp/r + Rpp) /.
    {R → solAllRTemp[[1]], Rp → solAllRTemp[[2]], Rpp → solAllRTemp[[3]]}],
  {r, 1, 30}, WorkingPrecision → 35, PlotRange → {-10^-20, 10^-20},
  MaxRecursion → 15, PlotPoints → 1000]
```

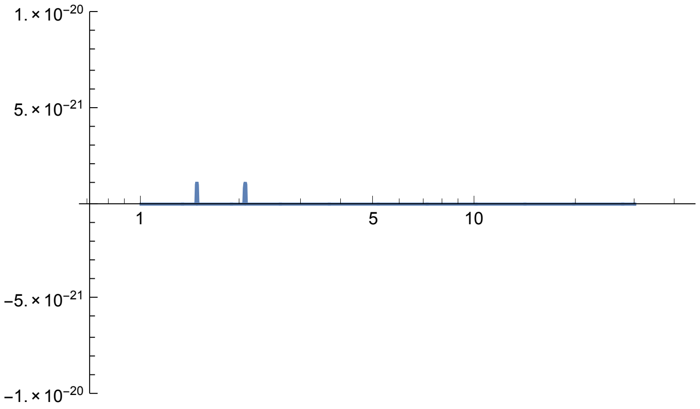


# Defining piecewise function

```
functionR[r1_] := Piecewise[{{(solAllRTemp[[1]] /. r → r1), rTrans > r1},
    {RAsymNew[orderAsym][r1], r1 ≥ rTrans}}]
```

```
functiondRdt[r1_] := Piecewise[{{(solAllRTemp[[2]] /. r → r1), rTrans > r1},
    {RAsymNew[orderAsym]'[r1], r1 ≥ rTrans}}]
```

```
(solAllRTemp[[1]]) - RAsymNew[orderAsym][r] /. {r → rTrans}
```

$0. \times 10^{-22}$

```
Plot[Evaluate[{(solAllRTemp[[1]]) - RAsymNew[orderAsym][r]}],
  {r, 0.9 rTrans, 1.1 rTrans}, PlotRange → All, WorkingPrecision → 30]
```

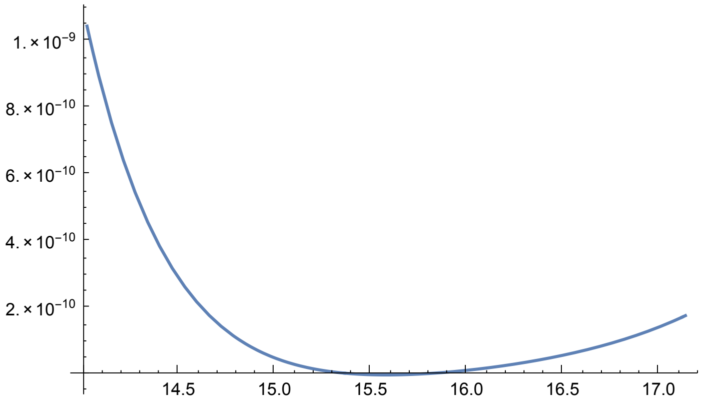

```
Plot[Evaluate[functionR[r]], {r, 0, 20}, PlotRange → All]
```

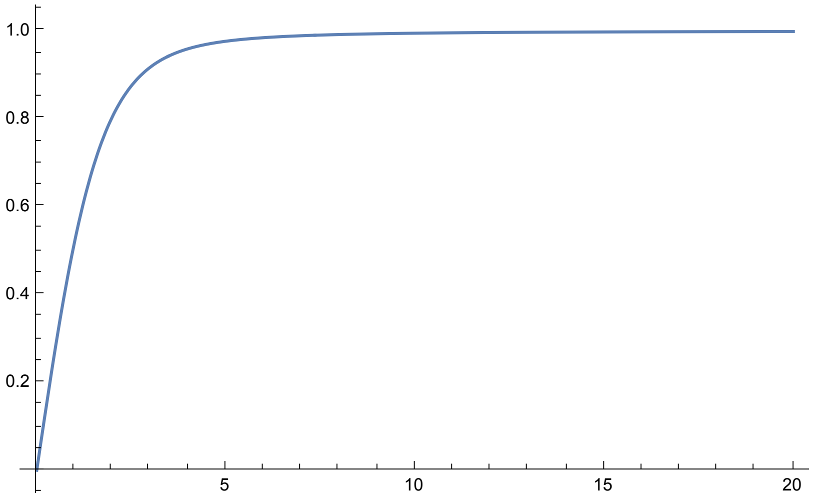


```
Plot[Evaluate[{functiondRdt[r] - functionR'[r]}],
 {r, 0.001, 1}, PlotRange → {-10^-10, 10^-10}]
```

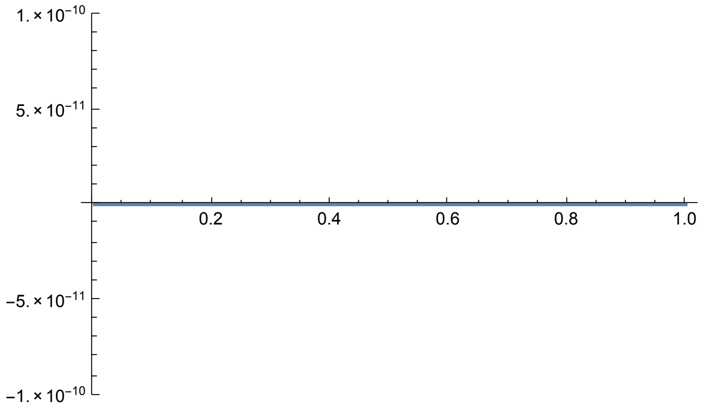


## Plots of accurate solution versus Pade:

```
Plot[Evaluate[{functiondRdt[r], RPade'[r]}], {r, 2, 4}, PlotRange → All]
```

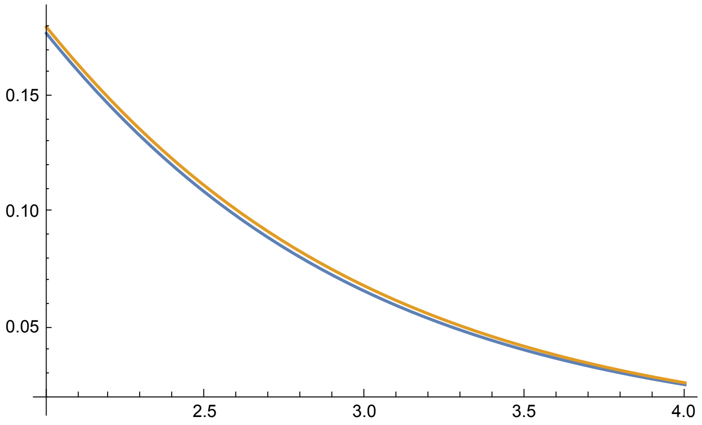

```
Plot[Evaluate[{functionR[r], RPade[r]}], {r, 2, 4}, PlotRange → All]
```

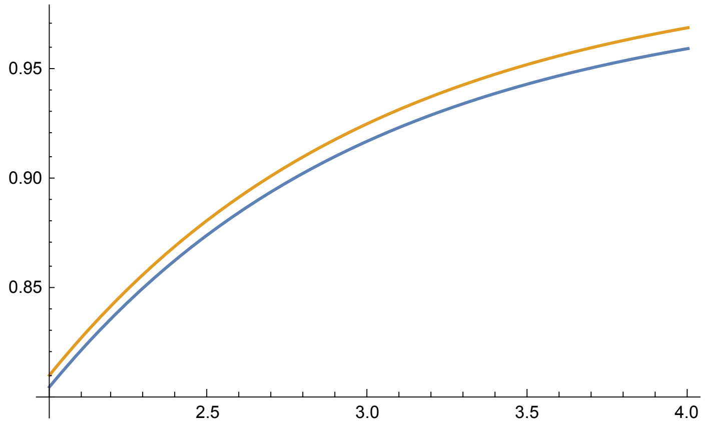


```
Plot[Evaluate[{functionR[r], RPade[r]}], {r, 10^(-4), 10^(2)},
 PlotRange → All, MaxRecursion → 3, PlotPoints → 10, Ticks →
  {{{10^-4, "10^-4"}, {10^-2, "10^-2"}, 1, {100, "10^2"}, {10000, "10^4"}}, Automatic},
 AxesStyle → {{Thick}, {Thick}}, TicksStyle → Thick,
 PlotStyle → {AbsoluteThickness[5]}, AxesLabel → {"r", "R(r)"},
 LabelStyle → Directive[Black, Large]]
```

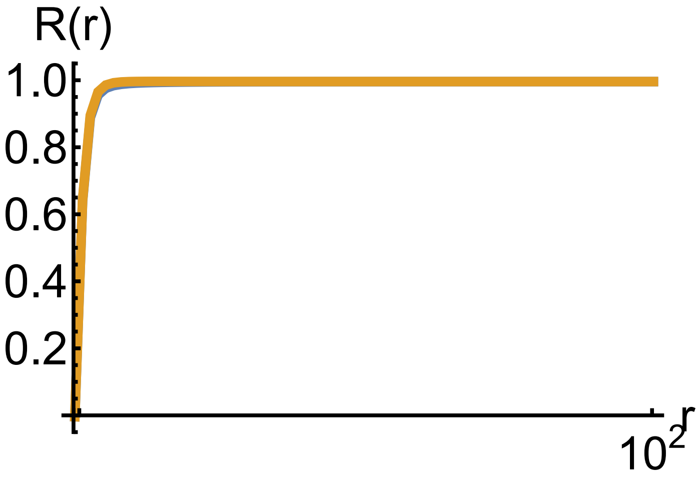


## Error between the integrands from accurate solution and Pade approximation:

```
Plot[Evaluate[{functiondRdt[r] - RPade'[r]}], {r, 0, 20}, PlotRange → {-10^-2, 10^-2}]
```

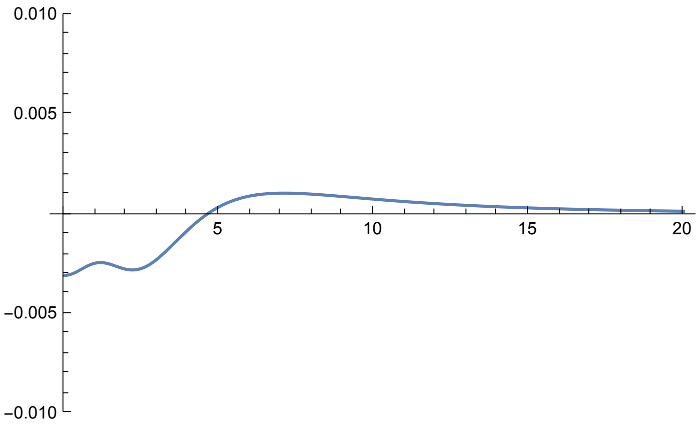

```
Plot[Evaluate[{functiondRdt[r] - RPade'[r]}],
 {r, 0.99 rTrans, 1.01 rTrans}, PlotRange → {-10^-4, 5 * 10^-4}]
```

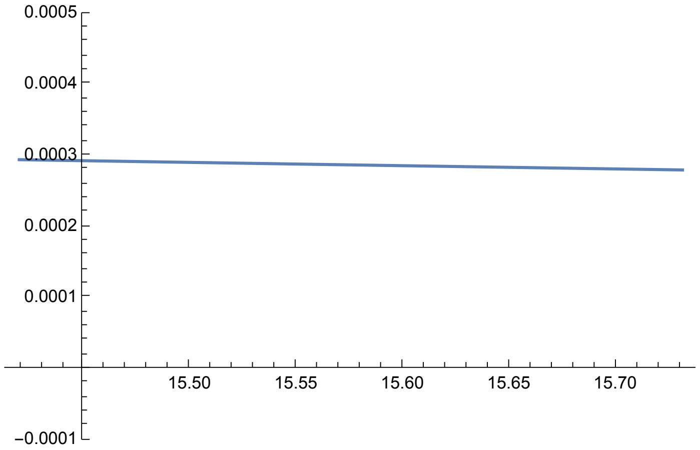


```
Plot[Evaluate[{functiondRdt[r] / RPade'[r] - 1}],
 {r, 2, 4}, PlotRange → {-10^-1, 10^-1}]
```

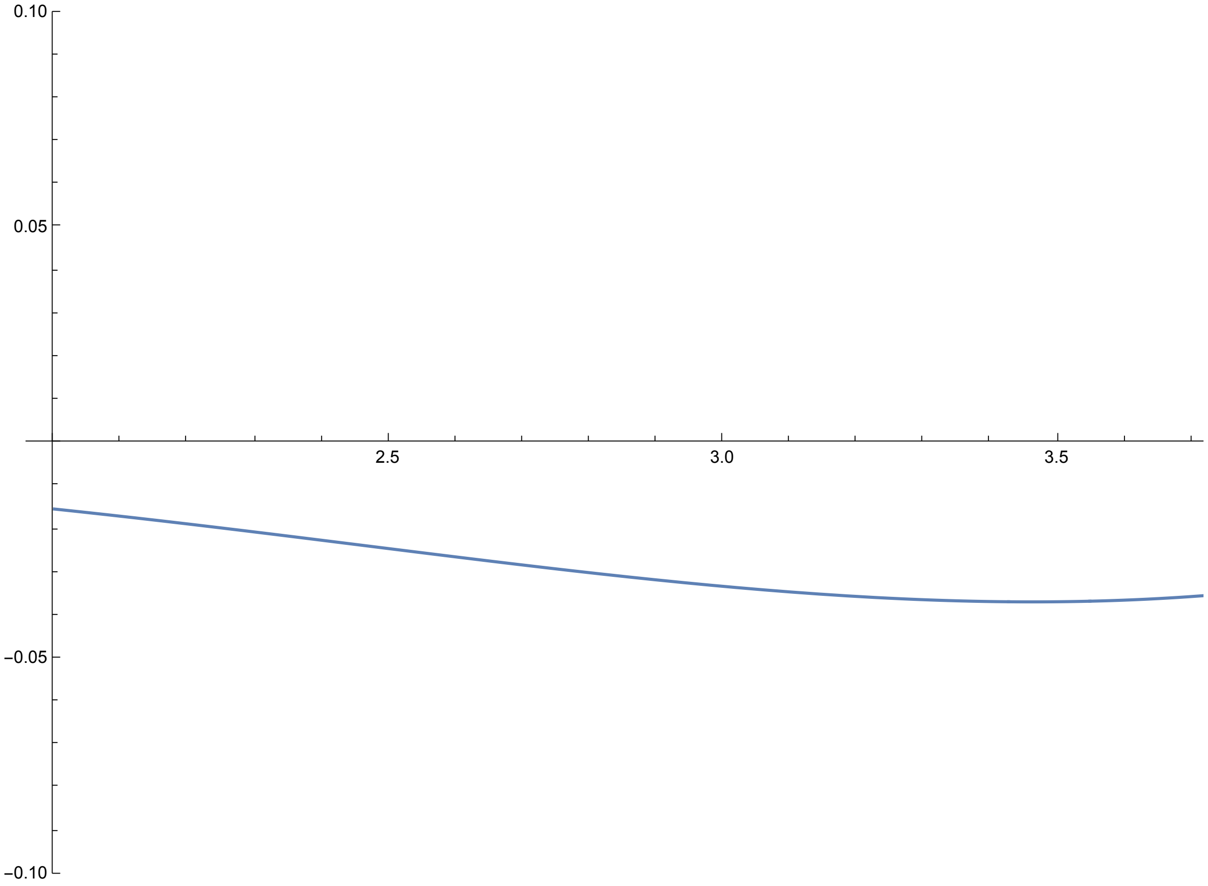

## Plotting Jump in the derivative of piecewise vortex profile R(r):

```
Plot[Evaluate[{functiondRdt[r]}],
 {r, 0.99999999999 rTrans, 1.00000000001 rTrans}, PlotRange → All]
```

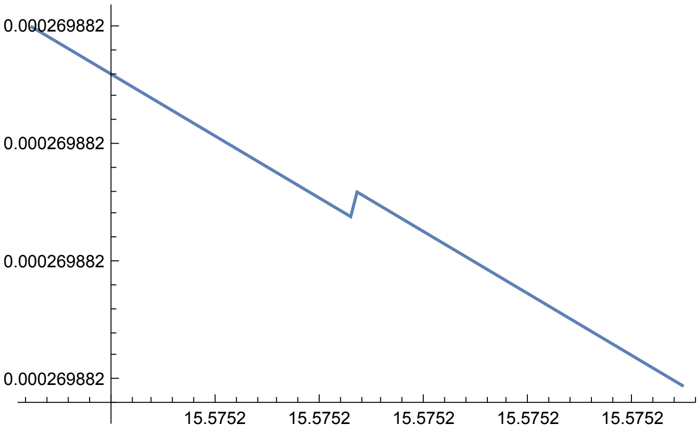


```
Plot[Evaluate[{functiondRdt[r]}], {r, 0, 20}, PlotRange → All]
```

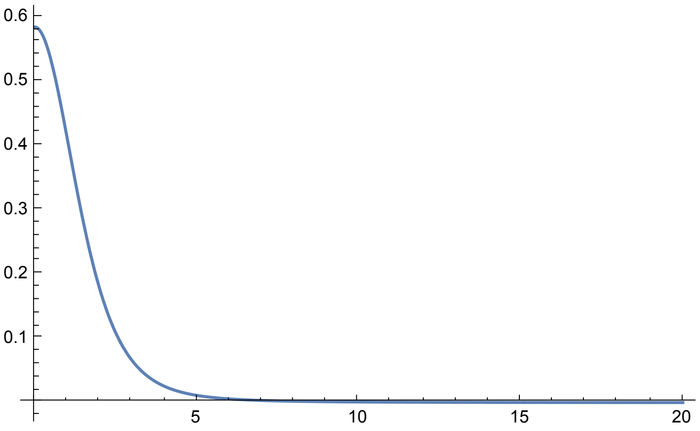


## Error of asymptotic solution at r = $r_{trans}$:

```
Evaluate[(R[r] - R[r]/r^2 - R[r]^3 + R'[r]/r + R''[r]) /. {R → functionR} /. r → rTrans]
```

$-1.9449451089356 \times 10^{-10}$

```
Plot[Evaluate[(R[r] - R[r]/r^2 - R[r]^3 + R'[r]/r + R''[r]) /. {R → functionR}],
 {r, 10^-10, 30}, WorkingPrecision → 30, PlotRange → All]
```

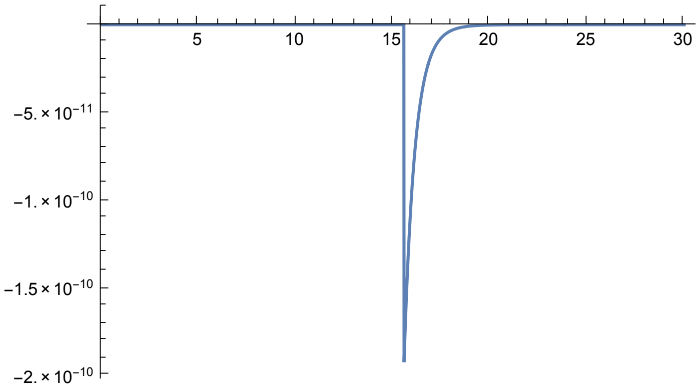


```
Plot[Evaluate[(R[r] - R[r]/r^2 - R[r]^3 + R'[r]/r + R''[r]) /. {R → functionR}],
 {r, 21, 30}, WorkingPrecision → 30, PlotRange → All]
```

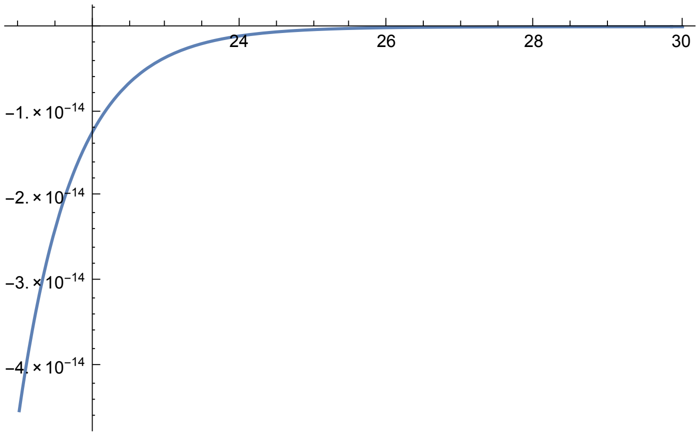


## Checking integrals of the piecewise function:

### Example 1: Integral of R’[r] from r=0 to r=∞ (should be equal to 1): We see no difference between our accurate solution and Pade approximation, both OK within round-off error $(10^{-15})$.

```
AbsoluteTiming[NIntegrate[Evaluate[functiondRdt[r1]],
  {r1, 10^-17, Infinity}, AccuracyGoal → 10, PrecisionGoal → 10, Method →
   {"GlobalAdaptive", "MaxErrorIncreases" → 10000}, Exclusions → r1 == rTrans]]
```

```
{21.133432, 1.}
```

```
1 - %[[2]]
```

$-1.11022 \times 10^{-15}$

```
NIntegrate[Evaluate[RPade'[r1]], {r1, 0, Infinity}, AccuracyGoal → 10,
 PrecisionGoal → 10, Method → {"GlobalAdaptive", "MaxErrorIncreases" → 10 000}]
```

1.

```
1 - %
```

$-1.9984\times10^{-15}$

### Example 2: Roberts' (2003) identity: Pade approximation gives a relative error of over 6%. Our accurate solution gives a relative error of about $10^{-9}$ %.

```
fRobTest = NIntegrate[Evaluate[(1 - (R[r])^2)^2 r /. R → functionR],
  {r, 10^-17, Infinity}, AccuracyGoal → 10, PrecisionGoal → 10, Method →
   {"GlobalAdaptive", "MaxErrorIncreases" → 10 000}, Exclusions → r == rTrans]
```

1.

```
1 - fRobTest
```

$1.41483\times10^{-11}$

```
fRobTestPade = NIntegrate[Evaluate[(1 - (R[r])^2)^2 r /. R → RPade],
  {r, 10^-17, Infinity}, AccuracyGoal → 10, PrecisionGoal → 10, Method →
   {"GlobalAdaptive", "MaxErrorIncreases" → 10 000}, Exclusions → r == rTrans]
```

0.936654

```
1 - fRobTestPade
```

0.0633465

### Example 3: $\mu_0$ as in the paper.

```
μ0 = 1 / 2 + NIntegrate[Evaluate[((R'[r])^2) * r /. R → functionR],
   {r, 10^-17, Infinity}, AccuracyGoal → 10, PrecisionGoal → 10, Method →
    {"GlobalAdaptive", "MaxErrorIncreases" → 10 000}, Exclusions → r == rTrans]
```

0.779091

## Numerical computation of cut-off length $\xi_*$

```
Clear[ξstar]
```

```
ξstar[a_] := 1 / 2 Exp[-1 / 2 - NIntegrate[Evaluate[((R'[r])^2) * r /. R → functionR],
     {r, 10^-17, Infinity}, AccuracyGoal → 10, PrecisionGoal → 10, Method →
      {"GlobalAdaptive", "MaxErrorIncreases" → 10 000}, Exclusions → r == rTrans] -
    (NIntegrate[Evaluate[((R[r])^2) / r /. R → functionR], {r, 10^-17, a},
       AccuracyGoal → 10, PrecisionGoal → 10, Method → {"GlobalAdaptive",
         "MaxErrorIncreases" → 10 000}, Exclusions → r == rTrans] - Log[a])]
```

```
ξstar[10.]
```

0.33990707833427636`

```
ξstar[100.]
0.3416122081499921`
ξstar[1. * 10^4]
0.34162928918850394`
ξstar[1. * 10^6]
0.34162929089648003`
ξstar[1. * 10^8]
0.3416292908966524`
ξstar[1. * 10^10]
0.34162929089664995`
ξstar[1. * 10^12]
0.3416292908966548`
ξstar[1. * 10^14]
0.34162929089664873`
ξstar[1. * 10^16]
0.3416292908966548`
ξstar[1. * 10^18]
0.3416292908966475`
ξstar[1. * 10^20]
0.3416292908966427`
ξstarTemp = 0.341629290897
0.341629
```
